# Supplementary material for: A tutorial on optimal dynamic treatment regimes
Source: arXiv:2502.16988 source file (2025-10-10)
Supplement: Supplementary file 1 [file supplement_tutorial.pdf]

# Supplementary example code to ‘A tutorial on optimal dynamic treatment regimes’

Chunyu Wang and Brian DM Tom

## 1. Example code for simulation studies in Section 4.1

### Load packages

We firstly load the required R packages among which **DTRreg** (<https://CRAN.R-project.org/package=DTRreg>) works for Q-learning, A-learning and dWOLS, **htetree** (<https://CRAN.R-project.org/package=htetree>) works for the causal tree method.

```
library(DTRreg) ##package for Q-learning, A-learning and dWOLS.
library(htetree) ##package for the causal tree
library(rgenoud) ##package for optimization in IPW and AIPW
library(rpart) ##package for conventional classification and regression trees
library(rpart.plot) ##package for tree plot
library(TruncatedNormal) ##package for truncated normal distribution
###Define functions
expit=function(x) 1/(1+exp(-x))
```

### Generate data

Data is generated as follows.

```
set.seed(3)
n=1000
L1=rnorm(n,mean=450,sd=150)
A1=rbinom(n,1,expit(2-0.006*L1))
L2=rnorm(n,mean=1.25*L1,sd=60)
A2=rbinom(n,1,expit(0.8-0.004*L2))
Y=rnorm(n,mean=400+1.6*L1,sd=60)-((L1<=250)-A1)*(250-L1)-((L2<=360)-A2)*(720-2*L2)
data=data.frame(L1=L1,A1=A1,L2=L2,A2=A2,Y=Y)
```

For illustrative purposes only, we here keep the seed fixed and all statistical methods shown below are applied to the generated dataset under the fixed seed.

### Q-learning

To illustrate the backward induction procedure, we firstly show the self-written code for Q-learning followed by directly calling the function ‘DTRreg’ from package **DTRreg**. The standard error returned from ‘DTRreg’ for Q-learning is calculated by bootstrap.

```
lm_2_q=lm(Y~A2+A2:L2+L1+A1+A1:L1+L2)
psi_2_q=lm_2_q$coefficients[c(2,6)]
beta_2_q=lm_2_q$coefficients[-c(2,6)]
#design matrix for the blip function in stage 2
blip_mat2=rbind(numeric(n)+1,L2)
```

```

#design matrix for the treatment-free term in stage 2
trtfre_mat2_q=rbind(numeric(n)+1,L1,A1,L2,A1*L1)
##construct the value function which serves as the response variable in stage 1
V_2=(c(t(blip_mat2)%*%psi_2_q)>0)*c(t(blip_mat2)%*%psi_2_q)+t(trtfre_mat2_q)%*%beta_2_q
lm_1_q=lm(V_2~A1+A1:L1+L1)
psi_1_q=lm_1_q$coefficients[c(2,4)]
psi_q=c(psi_1_q,psi_2_q)
psi_q

##          A1          A1:L1          A2          A2:L2
## 132.4566069  -0.7235409 467.9536090  -1.5184157

#use package
blip.mod=list(~L1,~L2)
treat.mod=list(A1~L1,A2~L2)
tf.mod=list(~L1, ~L1+A1+A1:L1+L2)
res_DTR_q=DTRreg(Y, blip.mod, treat.mod,tf.mod,data=data,method = "qlearn",var.estim = "bootstrap")
summary(res_DTR_q)

## DTR estimation over 2 stages:
##
## Blip parameter estimates
## Stage 1 (n = 1000)
##      Estimate Std_Error X95._CI_Lower X95._CI_Upper
## A1      132.4566    21.7308      89.8642     175.0490
## L1:A1    -0.7235     0.0485     -0.8186     -0.6285
## Stage 2 (n = 1000)
##      Estimate Std_Error X95._CI_Lower X95._CI_Upper
## A2      467.9536    41.6770     386.2668     549.6405
## L2:A2    -1.5184     0.0799     -1.6751     -1.3617
##
## Warning: possible non-regularity at stages 1, 2 (probs = 0.117, 0.170, respectively)
## Recommended dynamic treatment regimen:
## Stage 1: treat if 132.4566 - 0.7235 L1:A1 > 0
## Stage 2: treat if 467.9536 - 1.5184 L2:A2 > 0

```

## A-learning

- **A1:** A-learning without the treatment-free term.

Since the function ‘DTRreg’ does not allow for a null model for the treatment-free term, we wrote the following R code for A1, which is intended to solve the estimating equations:

$$\sum_{i=1}^n R_{ji} [\tilde{V}_{j+1,i}^A - A_{ji} R_{ji}^\top \psi_j] [A_{ji} - \mathbb{E}(A_{ji} | H_{ji}; \hat{\alpha}_j)] = 0, \quad j = 1, 2;$$

with  $R_{ji} = (1, L_{ji})^\top$  for  $j = 1, 2$  and  $i = 1, \dots, n$ ; from which we can get the closed form of  $\hat{\psi}_j$  as follows

$$\hat{\psi}_j = \left[ \sum_{i=1}^n R_{ji} \underbrace{A_{ji} [A_{ji} - \mathbb{E}(A_{ji} | H_{ji}; \hat{\alpha}_j)]}_{W_j} R_{ji}^\top \right]^{-1} \left( \sum_{i=1}^n R_{ji} [A_{ji} - \mathbb{E}(A_{ji} | H_{ji}; \hat{\alpha}_j)] \tilde{V}_{j+1,i}^A \right).$$

```

trt_1=glm(A1~L1,family = binomial)
trt_2=glm(A2~L2,family = binomial)

```

```

pre_trt_1=predict(trt_1,type = "response")
pre_trt_2=predict(trt_2,type = "response")
##stage 2
W2=(A2-pre_trt_2)*A2
blip_mat2=rbind(numeric(n)+1,L2)
trt_mat2=blip_mat2
est_mat2=tcrossprod(t(t(trt_mat2)*W2),blip_mat2)
est_vec2=rowSums(t(t(trt_mat2)*((A2-pre_trt_2)*Y)))
psi_2=solve(est_mat2,est_vec2)
### stage 1
W1=(A1-pre_trt_1)*A1
blip_mat1=rbind(numeric(n)+1,L1)
trt_mat1=blip_mat1
est_mat1=tcrossprod(t(t(trt_mat1)*W1),blip_mat1)
reg_2=((psi_2[1]+psi_2[2]*L2)>=0)-A2*(psi_2[1]+psi_2[2]*L2)
est_vec1=rowSums(t(t(trt_mat1)*((A1-pre_trt_1)*(Y+reg_2))))
psi_1=solve(est_mat1,est_vec1)
psi=c(psi_1,psi_2)
psi

```

```

##                L1                L2
## 289.331309   -1.096023 579.346860   -1.748558

```

And the standard error of estimates from A1 can be calculated by the sandwich variance estimator as follows.

```

#standard error of the estimate of psi_2 from A1
R_out2=c(Y-A2*t(blip_mat2)%*%psi_2)
R_trt2=A2-pre_trt_2
U_psi2=matrix(c(R_out2*R_trt2,(R_out2*R_trt2)*L2),nrow=2,ncol=n,byrow = TRUE)
W2_var=R_out2*pre_trt_2*(1-pre_trt_2)
U_psi2_d_alpha2=-tcrossprod(t(t(blip_mat2)*W2_var),trt_mat2)/n
U_alpha2_d_alpha2=-tcrossprod(t(t(trt_mat2)*(pre_trt_2*(1-pre_trt_2))),trt_mat2)/n
U_alpha2=matrix(c(R_trt2,R_trt2*L2),nrow=2,ncol=n,byrow = TRUE)
U_psi2_adj=U_psi2-U_psi2_d_alpha2%*%solve(U_alpha2_d_alpha2)%*%U_alpha2
meat_2=tcrossprod(U_psi2_adj)/n
U_psi2_d_psi2=-tcrossprod(t(t(blip_mat2)*(A2*R_trt2)),trt_mat2)/n
bread_2=solve(U_psi2_d_psi2)
var_psi2=bread_2%*%meat_2%*%t(bread_2)/n
sd_psi2=sqrt(diag(var_psi2))
sd_psi2

```

```

##                L2
## 95.6532376   0.1830657

```

```

#standard error of the estimate of psi_1 from A1
R_out1=c(Y+reg_2-A1*t(blip_mat1)%*%psi_1)
R_trt1=A1-pre_trt_1
U_psi1=matrix(c(R_out1*R_trt1,(R_out1*R_trt1)*L1),nrow=2,ncol=n,byrow = TRUE)
U_psi1_d_psi1=-tcrossprod(t(t(blip_mat1)*(A1*R_trt1)),trt_mat1)/n

W1_var=R_out1*pre_trt_1*(1-pre_trt_1)
U_psi1_d_alpha1=-tcrossprod(t(t(blip_mat1)*W1_var),trt_mat1)/n
U_alpha1_d_alpha1=-tcrossprod(t(t(trt_mat1)*(pre_trt_1*(1-pre_trt_1))),trt_mat1)/n
U_alpha1=matrix(c(R_trt1,R_trt1*L1),nrow=2,ncol=n,byrow = TRUE)

```

```

U_psi1_d_psi2=tcrossprod(t(t(blip_mat1)*(((psi_2[1]+psi_2[2]*L2)>=0)-A2)*R_trt1)),
                      blip_mat2)/n

U_psi1_adj=U_psi1-U_psi1_d_psi2**bread_2**U_psi2_adj-U_psi1_d_alpha1**
solve(U_alpha1_d_alpha1)**U_alpha1
meat_1=tcrossprod(U_psi1_adj)/n
bread_1=solve(U_psi1_d_psi1)
var_psi1=bread_1**meat_1**t(bread_1)/n
sd_psi1=sqrt(diag(var_psi1))
sd_psi1

##                               L1
## 88.9614841  0.2099044

```

- **A2:** regression adjustment for propensity score; that is, the OLS regression of  $\tilde{V}_{j+1}^A$  on  $A_j R_j$  and  $\mathbb{E}(A_j | H_j, \hat{\alpha}_j) R_j$ . The estimate of  $\psi$  from A2 is given below.

```

lm_2=lm(Y~-1+A2+A2:L2+pre_trt_2+pre_trt_2:L2)
psi_2_lm=lm_2$coefficients[c(1,3)]
reg_2_lm=((psi_2_lm[1]+psi_2_lm[2]*L2)>=0)-A2*(psi_2_lm[1]+psi_2_lm[2]*L2)
lm_1=lm((Y+reg_2_lm)~-1+A1+A1:L1+pre_trt_1+pre_trt_1:L1)
psi_1_lm=lm_1$coefficients[c(1,3)]
psi_lm=c(psi_1_lm,psi_2_lm)
psi_lm

```

```

##           A1      A1:L1      A2      A2:L2
## 292.036884 -1.142773 776.810062 -2.089843

```

And the standard error is calculated as follows.

```

#standard error of the estimate of psi_2 from A2
eta2=lm_2$coefficients[-c(1,3)]
R_out2_lm=c(Y-A2*t(blip_mat2)**psi_2_lm-pre_trt_2*t(blip_mat2)**eta2)
U_psi2_lm=matrix(c(R_out2_lm*A2,R_out2_lm*(A2*L2)),nrow=2,ncol=n,byrow = TRUE)
U_psi2_d_psi2_lm=-tcrossprod(t(t(blip_mat2)*A2),blip_mat2)/n
U_psi2_d_eta2=-tcrossprod(t(t(blip_mat2)*(A2*pre_trt_2)),blip_mat2)/n
W2_var_lm=pre_trt_2*(1-pre_trt_2)*A2*c(t(blip_mat2)**eta2)
U_psi2_d_alpha2_lm=-tcrossprod(t(t(blip_mat2)*W2_var_lm),trt_mat2)/n

U_eta2=matrix(c(R_out2_lm*pre_trt_2,R_out2_lm*(pre_trt_2*L2)),nrow=2,
              ncol=n,byrow = TRUE)
U_eta2_d_eta2=-tcrossprod(t(t(blip_mat2)*(pre_trt_2^2)),blip_mat2)/n

eta2_mat=tcrossprod(t(t(blip_mat2)*(pre_trt_2^2)),blip_mat2)/n
eta2_vec=t(pre_trt_2*t(blip_mat2))**c(Y-A2*t(blip_mat2)**psi_2_lm)/n

eta2_d_psi2=-solve(eta2_mat)**(tcrossprod(t(t(blip_mat2)*(A2*pre_trt_2)),
                      blip_mat2)/n)

W_alpha2=pre_trt_2*(1-pre_trt_2)
eta2_d_alpha2_1=-solve(eta2_mat)**(tcrossprod(t(t(blip_mat2)*(2*pre_trt_2*W_alpha2)),
                      blip_mat2)/n)**solve(eta2_mat)**eta2_vec+
solve(eta2_mat)**t(W_alpha2*t(blip_mat2))**c(Y-A2*t(blip_mat2)**psi_2_lm)/n

eta2_d_alpha2_2=-solve(eta2_mat)**(tcrossprod(t(t(blip_mat2)*(2*pre_trt_2*W_alpha2*L2)),
                      blip_mat2)/n)**solve(eta2_mat)**eta2_vec+
solve(eta2_mat)**t(W_alpha2*L2*t(blip_mat2))**c(Y-A2*t(blip_mat2)**psi_2_lm)/n

```

```

eta2_d_alpha2=cbind(eta2_d_alpha2_1,eta2_d_alpha2_2)

U_psi2_adj_lm=U_psi2_lm-(U_psi2_d_alpha2_lm+U_psi2_d_eta2%%eta2_d_alpha2)%%
solve(U_alpha2_d_alpha2)%%U_alpha2-
U_psi2_d_eta2%%solve(U_eta2_d_eta2)%%U_eta2

meat_2_lm=tcrossprod(U_psi2_adj_lm)/n
bread_2_lm=solve(U_psi2_d_psi2_lm+U_psi2_d_eta2%%eta2_d_psi2)
var_psi2_lm=bread_2_lm%%meat_2_lm%%t(bread_2_lm)/n
sd_psi2_lm=sqrt(diag(var_psi2_lm))
sd_psi2_lm

##                               L2
## 101.9260631    0.2013194

#standard error of the estimate of psi_1 from A2
eta1_lm=lmc$coefficients[-c(1,3)]
R_out1_lm=c(Y+reg_2_lm-A1*t(blip_mat1)%%psi_1_lm-pre_trt_1*t(blip_mat1)%%eta1)
U_psi1_lm=matrix(c(R_out1_lm*A1,R_out1_lm*(A1*L1)),nrow=2,ncol=n,byrow = TRUE)
U_psi1_d_psi1_lm=-tcrossprod(t(t(blip_mat1)*A1),blip_mat1)/n
U_psi1_d_eta1=-tcrossprod(t(t(blip_mat1)*(A1*pre_trt_1)),blip_mat1)/n
W1_var_lm=pre_trt_1*(1-pre_trt_1)*A1*c(t(blip_mat1)%%eta1)
U_psi1_d_alpha1_lm=-tcrossprod(t(t(blip_mat1)*W1_var_lm),trt_mat1)/n

U_eta1=matrix(c(R_out1_lm*pre_trt_1,R_out1_lm*(pre_trt_1*L1)),nrow=2,
              ncol=n,byrow = TRUE)
U_eta1_d_eta1=-tcrossprod(t(t(blip_mat1)*(pre_trt_1^2)),blip_mat1)/n

eta1_mat=tcrossprod(t(t(blip_mat1)*(pre_trt_1^2)),blip_mat1)/n
eta1_vec=t(pre_trt_1*t(blip_mat1))%%c(Y+reg_2_lm-A1*t(blip_mat1)%%psi_1_lm)/n

eta1_d_psi1=-solve(eta1_mat)%%(tcrossprod(t(t(blip_mat1)*(A1*pre_trt_1)),blip_mat1)/n)
W_alpha1=pre_trt_1*(1-pre_trt_1)

eta1_d_alpha1_1=-solve(eta1_mat)%%(tcrossprod(t(t(blip_mat1)*(2*pre_trt_1*W_alpha1)),
                                              blip_mat1)/n)%%solve(eta1_mat)%%eta1_vec+
solve(eta1_mat)%%t(W_alpha1*t(blip_mat1))%%c(Y+reg_2_lm-A1*t(blip_mat1)%%
                                              psi_1_lm)/n

eta1_d_alpha1_2=-solve(eta1_mat)%%(tcrossprod(t(t(blip_mat1)*(2*pre_trt_1*W_alpha1*L1)),
                                              blip_mat1)/n)%%solve(eta1_mat)%%eta1_vec+
solve(eta1_mat)%%t(W_alpha1*L1*t(blip_mat1))%%c(Y+reg_2_lm-A1*t(blip_mat1)%%psi_1_lm)/n

eta1_d_alpha1=cbind(eta1_d_alpha1_1,eta1_d_alpha1_2)

U_psi1_d_psi2_lm=tcrossprod(t(t(blip_mat1)*(A1*((psi_2_lm[1]+psi_2_lm[2]*L2)>=0)-A2))),
                          blip_mat2)/n
eta1_d_psi2=solve(eta1_mat)%%tcrossprod(t(t(blip_mat1)*(pre_trt_1*
                                              (((psi_2_lm[1]+psi_2_lm[2]*L2)>=0)-A2))),blip_mat2)/n

U_psi1_adj_lm=U_psi1_lm-(U_psi1_d_alpha1_lm+U_psi1_d_eta1%%eta1_d_alpha1)%%
solve(U_alpha1_d_alpha1)%%U_alpha1-
(U_psi1_d_psi2_lm+U_psi1_d_eta1%%eta1_d_psi2)%%bread_2_lm%%U_psi2_adj_lm-
U_psi1_d_eta1%%solve(U_eta1_d_eta1)%%U_eta1

```

```

meat_1_lm=tcrossprod(U_psi1_adj_lm)/n
bread_1_lm=solve(U_psi1_d_psi1_lm+U_psi1_d_eta1%%eta1_d_psi1)

var_psi1_lm=bread_1_lm%%meat_1_lm%%t(bread_1_lm)/n
sd_psi1_lm=sqrt(diag(var_psi1_lm))
sd_psi1_lm

```

```

##                      L1
## 108.7860487    0.2493853

```

As the standard errors of the estimates from A1 and A2 are large, the values of  $\hat{\psi}_2$  and  $\hat{\psi}_1$  from A.1 and A.2 will vary a lot when changing the random seed. The results in Table 2 in the tutorial are obtained under 1000 Monte Carlo replications.

- **A3:** A-learning with the linear treatment-free term  $D_j^\top \xi_j$  with  $D_1 = (1, L_1)$  and  $D_2 = (1, L_1, A_1, L_1 A_1, L_2)$ . A3 can be implemented by using ‘DTRreg’ function a

```

blip.mod=list(~L1,~L2)
treat.mod=list(A1~L1,A2~L2)
tf.mod=list(~L1, ~L1+A1+A1:L1+L2)
res_DTR=DTRreg(Y, blip.mod, treat.mod,tf.mod, data=data,method = "gest",var.estim = "sandwich")
psi_dr=unlist(res_DTR$psi)
summary(res_DTR)

```

```

## DTR estimation over 2 stages:
##
## Blip parameter estimates
## Stage 1 (n = 1000)
##      Estimate Std_Error X95._CI_Lower X95._CI_Upper
## A1      212.8284    22.6375      168.4590      257.1979
## L1:A1    -0.9140     0.0507      -1.0134      -0.8146
## Stage 2 (n = 1000)
##      Estimate Std_Error X95._CI_Lower X95._CI_Upper
## A2      637.0245    46.1917      546.4887      727.5604
## L2:A2    -1.8455     0.0812      -2.0046      -1.6864
##
## Warning: possible non-regularity at stages 1, 2 (probs = 0.16, 0.20, respectively)
## Recommended dynamic treatment regimen:
## Stage 1: treat if 212.8284 - 0.9140 L1:A1 > 0
## Stage 2: treat if 637.0245 - 1.8455 L2:A2 > 0

```

- **A4:** regression adjustment for propensity score; i.e., the OLS regression of  $\tilde{V}_{j+1}^A$  on  $A_j R_j$ ,  $\mathbb{E}(A_j|H_j, \hat{\alpha}_j) R_j$  and  $D_j$ . The estimate of  $\psi$  from A4 is given below.

```

lm_2_dr=lm(Y~A2+A2:L2+pre_trt_2+pre_trt_2:L2+L1+A1+A1:L1+L2)
psi_2_lm_dr=lm_2_dr$coefficients[c(2,7)]
reg_2_lm_dr=((psi_2_lm_dr[1]+psi_2_lm_dr[2]*L2)>=0)-A2)*(psi_2_lm_dr[1]+psi_2_lm_dr[2]*L2)
lm_1_dr=lm((Y+reg_2_lm_dr)~A1+A1:L1+pre_trt_1+pre_trt_1:L1+L1)
psi_1_lm_dr=lm_1_dr$coefficients[c(2,5)]
psi_lm_dr=c(psi_1_lm_dr,psi_2_lm_dr)
psi_lm_dr

```

```

##          A1          A1:L1          A2          A2:L2
## 211.8236871 -0.9141127 691.3534432 -1.9393301

```

And the standard error is calculated as follows.

```

#standard error of the estimate of psi_2 from A4
xi_2_lm=lm_2_dr$coefficients[c(1,4,5,9,6)]
eta2_dr=lm_2_dr$coefficients[c(3,8)]
beta2=c(eta2_dr,xi_2_lm)

lm_psi2_mat=rbind(A2,A2*L2)
trtfre_mat2=rbind(numeric(n)+1,L1,A1,A1*L1,L2)
lm_beta2_mat=rbind(rbind(pre_trt_2,pre_trt_2*L2),trtfre_mat2)

R_out2_lm_dr=c(Y-t(lm_psi2_mat)%*%psi_2_lm_dr-t(lm_beta2_mat)%*%beta2)
U_psi2_lm_dr=matrix(c(R_out2_lm_dr*A2,R_out2_lm_dr*(A2*L2)),nrow=2,ncol=n,byrow = TRUE)
U_psi2_d_psi2_lm_dr=-tcrossprod(t(t(blip_mat2)*A2),blip_mat2)/n
U_psi2_d_beta2=-tcrossprod(lm_psi2_mat,lm_beta2_mat)/n
W2_var_lm_dr=pre_trt_2*(1-pre_trt_2)*A2*c(t(blip_mat2)%*%eta2_dr)
U_psi2_d_alpha2_lm_dr=-tcrossprod(t(t(blip_mat2)*W2_var_lm_dr),trt_mat2)/n

U_beta2=t(t(lm_beta2_mat)*R_out2_lm_dr)
U_beta2_d_beta2=-tcrossprod(lm_beta2_mat,lm_beta2_mat)/n

beta2_mat=tcrossprod(lm_beta2_mat,lm_beta2_mat)/n
beta2_vec=lm_beta2_mat%*%c(Y-A2*t(blip_mat2)%*%psi_2_lm_dr)/n
#solve(beta2_mat)%*%beta2_vec
beta2_d_psi2=-solve(beta2_mat)%*%(tcrossprod(lm_beta2_mat,lm_psi2_mat)/n)

W_alpha2=pre_trt_2*(1-pre_trt_2)
d_alpha2_1=rbind(rbind(W_alpha2,W_alpha2*L2),matrix(0,ncol=n,nrow=length(xi_2_lm)))
d_alpha2_2=rbind(rbind(W_alpha2*L2,W_alpha2*L2^2),matrix(0,ncol=n,nrow=length(xi_2_lm)))
mat_d_alpha2_1=tcrossprod(d_alpha2_1,lm_beta2_mat)/n
mat_d_alpha2_2=tcrossprod(d_alpha2_2,lm_beta2_mat)/n

beta2_d_alpha2_1=-solve(beta2_mat)%*%(mat_d_alpha2_1+t(mat_d_alpha2_1))%*%
solve(beta2_mat)%*%beta2_vec+
solve(beta2_mat)%*%d_alpha2_1%*%c(Y-A2*t(blip_mat2)%*%psi_2_lm_dr)/n

beta2_d_alpha2_2=-solve(beta2_mat)%*%(mat_d_alpha2_2+t(mat_d_alpha2_2))%*%
solve(beta2_mat)%*%beta2_vec+
solve(beta2_mat)%*%d_alpha2_2%*%c(Y-A2*t(blip_mat2)%*%psi_2_lm_dr)/n

beta2_d_alpha2=cbind(beta2_d_alpha2_1,beta2_d_alpha2_2)

U_psi2_adj_lm_dr=U_psi2_lm_dr-(U_psi2_d_alpha2_lm_dr+U_psi2_d_beta2%*%beta2_d_alpha2)%*%
solve(U_alpha2_d_alpha2)%*%U_alpha2-
U_psi2_d_beta2%*%solve(U_beta2_d_beta2)%*%U_beta2

meat_2_lm_dr=tcrossprod(U_psi2_adj_lm_dr)/n
bread_2_lm_dr=solve(U_psi2_d_psi2_lm_dr+U_psi2_d_beta2%*%beta2_d_psi2)
var_psi2_lm_dr=bread_2_lm_dr%*%meat_2_lm_dr%*%t(bread_2_lm_dr)/n
sd_psi2_lm_dr=sqrt(diag(var_psi2_lm_dr))
sd_psi2_lm_dr

```

```

##                               L2
## 16.30922517   0.02986879

```

```

#standard error of the estimate of psi_1 from A4
xi_1_lm=lm_1_dr$coefficients[c(1,4)]
eta1_dr=lm_1_dr$coefficients[c(3,6)]
beta1=c(eta1_dr,xi_1_lm)

lm_psi1_mat=rbind(A1,A1*L1)
trtfre_mat1=rbind(numeric(n)+1,L1)
lm_beta1_mat=rbind(rbind(pre_trt_1,pre_trt_1*L1),trtfre_mat1)

R_out1_lm_dr=c(Y+reg_2_lm_dr-t(lm_psi1_mat)%*%psi_1_lm_dr-t(lm_beta1_mat)%*%beta1)
U_psi1_lm_dr=matrix(c(R_out1_lm_dr*A1,R_out1_lm_dr*(A1*L1)),nrow=2,ncol=n,byrow = TRUE)
U_psi1_d_psi1_lm_dr=-tcrossprod(t(t(blip_mat1)*A1),blip_mat1)/n
U_psi1_d_beta1=-tcrossprod(lm_psi1_mat,lm_beta1_mat)/n
W1_var_lm_dr=pre_trt_1*(1-pre_trt_1)*A1*c(t(blip_mat1)%*%eta1_dr)
U_psi1_d_alpha1_lm_dr=-tcrossprod(t(t(blip_mat1)*W1_var_lm_dr),trtfre_mat1)/n

U_beta1=t(t(lm_beta1_mat)*R_out1_lm_dr)
U_beta1_d_beta1=-tcrossprod(lm_beta1_mat,lm_beta1_mat)/n

beta1_mat=tcrossprod(lm_beta1_mat,lm_beta1_mat)/n
beta1_vec=lm_beta1_mat%*%c(Y+reg_2_lm_dr-A1*t(blip_mat1)%*%psi_1_lm_dr)/n
beta1_d_psi1=-solve(beta1_mat)%*%(tcrossprod(lm_beta1_mat,lm_psi1_mat)/n)

W_alpha1=pre_trt_1*(1-pre_trt_1)
d_alpha1_1=rbind(rbind(W_alpha1,W_alpha1*L1),matrix(0,ncol=n,nrow=length(xi_1_lm)))
d_alpha1_2=rbind(rbind(W_alpha1*L1,W_alpha1*L1^2),matrix(0,ncol=n,nrow=length(xi_1_lm)))
mat_d_alpha1_1=tcrossprod(d_alpha1_1,lm_beta1_mat)/n
mat_d_alpha1_2=tcrossprod(d_alpha1_2,lm_beta1_mat)/n

beta1_d_alpha1_1=-solve(beta1_mat)%*%(mat_d_alpha1_1+t(mat_d_alpha1_1))%*%
solve(beta1_mat)%*%beta1_vec+
solve(beta1_mat)%*%d_alpha1_1%*%c(Y+reg_2_lm_dr-A1*t(blip_mat1)%*%psi_1_lm_dr)/n
beta1_d_alpha1_2=-solve(beta1_mat)%*%(mat_d_alpha1_2+t(mat_d_alpha1_2))%*%
solve(beta1_mat)%*%beta1_vec+
solve(beta1_mat)%*%d_alpha1_2%*%c(Y+reg_2_lm_dr-A1*t(blip_mat1)%*%psi_1_lm_dr)/n
beta1_d_alpha1=cbind(beta1_d_alpha1_1,beta1_d_alpha1_2)

U_psi1_d_psi2_lm_dr=tcrossprod(t(t(blip_mat1)*(A1*((psi_2_lm_dr[1]+
psi_2_lm_dr[2]*L2)>=0)-A2))),blip_mat2)/n
beta1_d_psi2=solve(beta1_mat)%*%tcrossprod(t(t(lm_beta1_mat)*((psi_2_lm_dr[1]+
psi_2_lm_dr[2]*L2)>=0)-A2))),blip_mat2)/n

U_psi1_adj_lm_dr=U_psi1_lm_dr-(U_psi1_d_alpha1_lm_dr+U_psi1_d_beta1%*%beta1_d_alpha1)%*%
solve(U_alpha1_d_alpha1)%*%U_alpha1-
U_psi1_d_beta1%*%solve(U_beta1_d_beta1)%*%U_beta1-
(U_psi1_d_psi2_lm_dr+U_psi1_d_beta1%*%beta1_d_psi2)%*%bread_2_lm_dr%*%U_psi2_adj_lm_dr

meat_1_lm_dr=tcrossprod(U_psi1_adj_lm_dr)/n
bread_1_lm_dr=solve(U_psi1_d_psi1_lm_dr+U_psi1_d_beta1%*%beta1_d_psi1)
var_psi1_lm_dr=bread_1_lm_dr%*%meat_1_lm_dr%*%t(bread_1_lm_dr)/n
sd_psi1_lm_dr=sqrt(diag(var_psi1_lm_dr))
sd_psi1_lm_dr

```

```
##
```

```
L1
```



```
## 15.88453728 0.03713973
```

- **dWOLS**: dynamic weighted OLS developed by (Wallace and Moodie 2015), which is included in the package.

```
res_DTR_w=DTRreg(Y, blip.mod, treat.mod,tf.mod,data=data,method = "dwols",
                 var.estim = "bootstrap")
psi_wols=unlist(res_DTR_w$psi)
summary(res_DTR_w)
```

```
## DTR estimation over 2 stages:
```

```
##
```

```
## Blip parameter estimates
```

```
## Stage 1 (n = 1000)
```

```
##      Estimate Std_Error X95._CI_Lower X95._CI_Upper
## A1      212.4846   21.3532      170.6323      254.3369
## L1:A1   -0.9130    0.0498       -1.0106       -0.8153
```

```
## Stage 2 (n = 1000)
```

```
##      Estimate Std_Error X95._CI_Lower X95._CI_Upper
## A2      640.1430   40.1432      561.4623      718.8237
## L2:A2   -1.8541    0.0679       -1.9872       -1.7209
```

```
##
```

```
## Warning: possible non-regularity at stages 1, 2 (probs = 0.153, 0.165, respectively)
```

```
## Recommended dynamic treatment regimen:
```

```
## Stage 1: treat if 212.4846 - 0.9130 L1:A1 > 0
```

```
## Stage 2: treat if 640.1430 - 1.8541 L2:A2 > 0
```

## Causal Tree

```
pro_trt2=mean(A2)
ipt2=ifelse(A2==1,pro_trt2/pre_trt_2,(1-pro_trt2)/(1-pre_trt_2))

tree2ipw=causalTree(Y~L2, treatment = A2, data=data, weights = ipt2,
                   split.Rule = "CT", cv.option = "CT", split.Honest = T,
                   cv.Honest = T, split.Bucket = T,
                   xval = 5, cp = 0, minsize = 10,bucketMax = 20)

rpart.plot(tree2ipw)
```

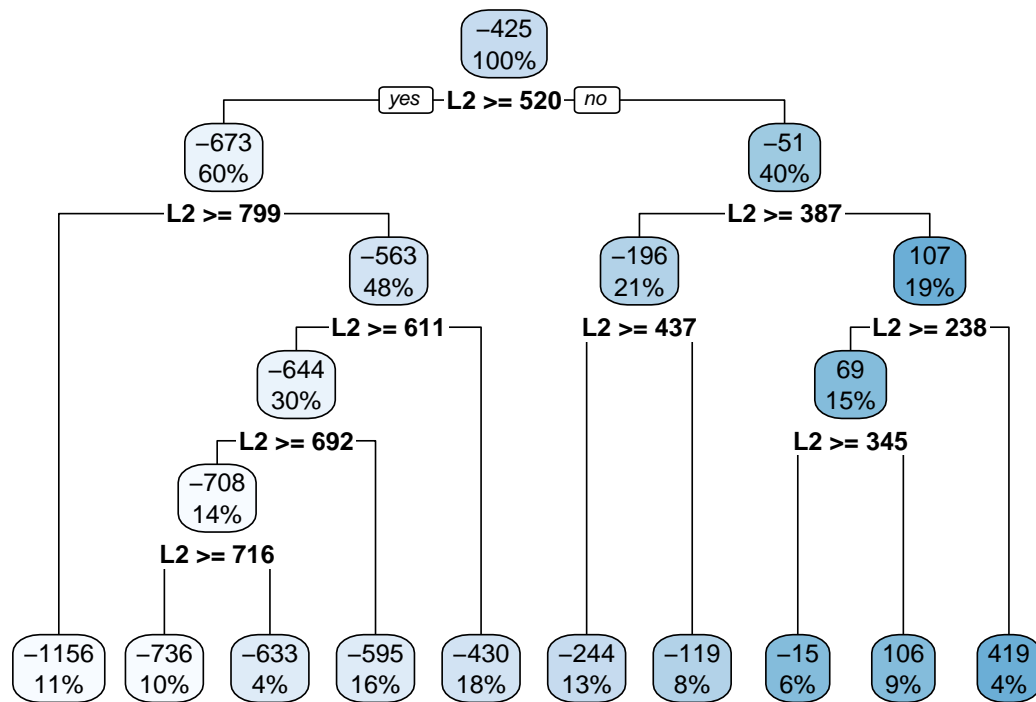

```

contra2=predict(tree2ipw)

Y_opt2=data$Y+((contra2>0)-data$A2)*contra2
data$Y_opt2=Y_opt2
pro_trt1=mean(A1)
ipt1=ifelse(A1==1,pro_trt1/pre_trt_1,(1-pro_trt1)/(1-pre_trt_1))
tree1ipw=causalTree(Y_opt2~L1, treatment = A1, data=data,weights = ipt1,
  split.Rule = "CT", cv.option = "CT", split.Honest = T,
  cv.Honest = T, split.Bucket = T,
  xval = 5, cp = 0,minsize=5,bucketMax = 20)
rpart.plot(tree1ipw)

```

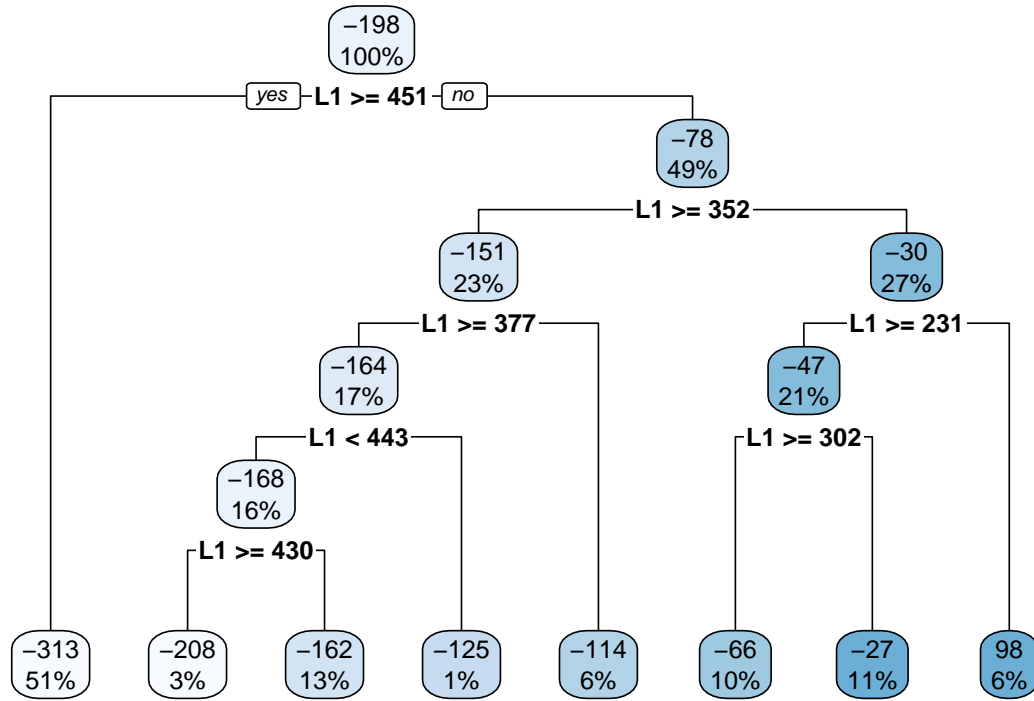

Note that *weights* specified in ‘causalTree’ is to correct for variations in propensity scores inside the leaf when the leaves are not small enough. Besides the inverse probability weighting used above,  $|A_j - \mathbb{E}[A_j|H_j]|$  can also be used as the weights to correct for bias due to confounding.

## IPWE

The objective function  $\text{IPWE}(\psi)$  is defined as follows.

```

est.ipw=function(data){
  n=dim(data)[1]
  #### Estimate propensity score
  trt_1=glm(data$A1~data$L1,family = binomial)
  trt_2=glm(data$A2~data$L2,family = binomial)
  pre_trt_2=predict(trt_2,type = "response")
  pre_trt_1=predict(trt_1,type = "response")

  blip_mat2=rbind(numeric(n)+1,data$L2)
  blip_mat1=rbind(numeric(n)+1,data$L1)

  objfun_ipw=function(par){

    psi_1_ipw=c(par[1],-1)
    #psi_1_ipw=par[1:2]
    psi_2_ipw=c(par[2],-1)
    #psi_2_ipw=par[3:4]

    ###indicator: whether the observed treatment sequence is consistent with
    ### the treatment regime indexed by psi
  }
}

```

```

    contra1_ipw=c(t(blip_mat1)%*%psi_1_ipw)
    contra2_ipw=c(t(blip_mat2)%*%psi_2_ipw)
    consis_categor=as.numeric(data$A1==as.numeric(contra1_ipw>0))+
      as.numeric(data$A2==as.numeric(contra2_ipw>0))
    consis_ind=as.numeric(consis_categor==2)
    consis_pro=ifelse(contra1_ipw>0,pre_trt_1,1-pre_trt_1)*
      ifelse(contra2_ipw>0,pre_trt_2,1-pre_trt_2)
    marmean_poten_ipw=sum(data$Y[consis_ind==1]/consis_pro[consis_ind==1])/n
    return(marmean_poten_ipw)
  }

  low_bou=c(0,0)
  upp_bou=c(max(data$L1),max(data$L2))

  res_ipw=tryCatch(genoud(objfun_ipw,max=TRUE,nvars =2,pop.size = 1000,
    starting.values = c(mean(data$L1),mean(data$L2)),
    Domains = cbind(low_bou,upp_bou),
    optim.method = "Nelder-Mead",print.level=0),
    warning=function(x) return(NULL))

  if(is.null(res_ipw)){
    return(list(thresh_1_aipw=0,thresh_2_aipw=0))
  }

  par_ipw=res_ipw$par

  thresh_1_ipw=par_ipw[1]
  thresh_2_ipw=par_ipw[2]

  return(list(thresh_1_ipw=thresh_1_ipw,thresh_2_ipw=thresh_2_ipw))
}

```

And IPWE is the value of parameters which maximizes  $\text{IPWE}(\psi)$  over the feasible set.

```

psi_ipw=unlist(est.ipw(data))
psi_ipw

```

```

## thresh_1_ipw thresh_2_ipw
##      143.9401      272.7070

```

## AIPWE

The objective function  $\text{AIPWE}(\psi)$  is defined as follows.

```

est.aipw=function(data){
  n=dim(data)[1]
  ##### Estimate propensity score
  trt_1=glm(data$A1~data$L1,family = binomial)
  trt_2=glm(data$A2~data$L2,family = binomial)
  pre_trt_2=predict(trt_2,type = "response")
  pre_trt_1=predict(trt_1,type = "response")

```

```

blip_mat2=rbind(numeric(n)+1,data$L2)
blip_mat1=rbind(numeric(n)+1,data$L1)

### AIPW
objfun_aipw=function(par){

  psi_1_aipw=c(par[1],-1)
  psi_2_aipw=c(par[2],-1)

  contra1_aipw=c(t(blip_mat1)%*%psi_1_aipw)
  contra2_aipw=c(t(blip_mat2)%*%psi_2_aipw)

  ###categorical variable: 1(fails to match in stage 1)/2 (matched in stage 1 but fails in stage 2),
  consis_categor_aipw=ifelse(data$A1!=as.numeric(contra1_aipw>0),1,
                             ifelse(data$A2!=as.numeric(contra2_aipw>0),2,3))
  ###this is a simple case because pro(A2|L2,...) does not depend on A1
  ###hazard: fail to match at the kth stage given it matches through k-1 stages.
  haz1=ifelse(contra1_aipw>0,1-pre_trt_1,pre_trt_1)
  haz2=numeric(n)+1
  haz2[consis_categor_aipw>1]=ifelse(contra2_aipw[consis_categor_aipw>1]>0,
                                     1-pre_trt_2[consis_categor_aipw>1],
                                     pre_trt_2[consis_categor_aipw>1])

  ####prob_k=prob(consis_categor_aipw>k)
  prob_1=1-haz1
  prob_2=numeric(n)+1
  prob_2[consis_categor_aipw>=2]=(1-haz1[consis_categor_aipw>=2])*(1-haz2[consis_categor_aipw>=2])

  ####augment terms
  lm_2_q=lm(Y~A2+A2:L2+L1+A1+A1:L1+L2,data=data)
  trtfre_mat2_q=rbind(numeric(n)+1,data$L1,data$A1,data$L2,data$A1*data$L1)
  psi_2_q=lm_2_q$coefficients[c(2,6)]
  beta_2_q=lm_2_q$coefficients[-c(2,6)]
  V_2=(c(t(blip_mat2)%*%psi_2_q)>0)*c(t(blip_mat2)%*%psi_2_q)+t(trtfre_mat2_q)%*%beta_2_q
  lm_1_q=lm(V_2~A1+A1:L1+L1,data=data)
  newdata_1=data.frame(L1=data$L1,A1=as.numeric(contra1_aipw>0))
  newdata_2=data.frame(L1=data$L1,A1=as.numeric(contra1_aipw>0),
                       L2=data$L2,A2=as.numeric(contra2_aipw>0))

  aug1=(as.numeric(consis_categor_aipw==1)-haz1)/prob_1*predict(lm_1_q,newdata_1)
  aug2=numeric(n)
  aug2[consis_categor_aipw>1]=(as.numeric(consis_categor_aipw[consis_categor_aipw>1]==2)-
                              haz2[consis_categor_aipw>1])/prob_2[consis_categor_aipw>1]*
    predict(lm_2_q,newdata_2[consis_categor_aipw>1,])

  marmean_poten_aipw=sum(data$Y[consis_categor_aipw==3]/prob_2[consis_categor_aipw==3])/n+
    sum(aug1+aug2)/n

  return(marmean_poten_aipw)
}

low_bou=c(0,0)

```

```

upp_bou=c(max(data$L1),max(data$L2))

res_aipw=tryCatch(genoud(objfun_aipw,max=TRUE,nvars = 2,pop.size = 1000,
  starting.values = c(mean(data$L1),mean(data$L2)),
  Domains = cbind(low_bou,upp_bou),
  optim.method = "Nelder-Mead",print.level=0),
  warning=function(x) return(NULL))

if(is.null(res_aipw)){
  return(list(thresh_1_aipw=0,thresh_2_aipw=0))
}

par_aipw=res_aipw$par

thresh_1_aipw=par_aipw[1]
thresh_2_aipw=par_aipw[2]

return(list(thresh_1_aipw=thresh_1_aipw,thresh_2_aipw=thresh_2_aipw))
}

```

And AIPWE is the value of parameters which maximizes  $AIPWE(\psi)$  over the feasible set.

```

psi_aipw=unlist(est.aipw(data))
psi_aipw

```

```

## thresh_1_aipw thresh_2_aipw
##      243.0565      381.4700

```

Assess the performance of  $\hat{d}^{\text{opt}}$  via  $\mathbb{E}[Y^*(\hat{d}^{\text{opt}})]$

For a given estimate of  $d^{\text{opt}}$ , say,  $\hat{d}^{\text{opt}}$  which is indexed by  $\hat{\psi}$ , the achieved average value of the outcome  $\mathbb{E}[Y^*(\hat{d}^{\text{opt}})]$  is calculated as follows.

```

mean.opt=function(par,B){ # parameters should be passed in order (psi_10,psi_11,psi_20,psi_21).
  L1_sam=rnorm(B,mean=450,sd=150)
  L2_sam=rnorm(B,mean=1.25*L1_sam,sd=60)
  reg1=((L1_sam<=250)-(par[1]+par[2]*L1_sam>0))*(250-L1_sam)
  reg2=((L2_sam<=360)-(par[3]+par[4]*L2_sam>0))*(720-2*L2_sam)
  Y=rnorm(B,mean=400+1.6*L1_sam,sd=60)-reg1-reg2
  return(mean(Y))
}

```

```

B=10000
mean.opt(c(250,-1,720,-2),B) ##True

```

```

## [1] 1121.815
mean.opt(c(psi_ipw[1],-1,psi_ipw[2],-1),B) ##IPWE

```

```

## [1] 1111.663
mean.opt(c(psi_aipw[1],-1,psi_aipw[2],-1),B) ##AIPWE

```

```

## [1] 1122.181

```

```
mean.opt(psi_q,B) ##Q-learning
```

```
## [1] 1120.315
```

```
mean.opt(psi_dr,B) ##A3
```

```
## [1] 1118.162
```

The achieved average value of the outcome  $\mathbb{E}[Y^*(\hat{d}^{\text{opt}})]$  under a tree method is calculated as follows.

```
mean.opt.tree=function(tree1,tree2,B){
  L1_sam=rnorm(B,mean=450,sd=150)
  L2_sam=rnorm(B,mean=1.25*L1_sam,sd=60)
  contra1_sam=predict(tree1,newdata = data.frame(L1=L1_sam))
  contra2_sam=predict(tree2,newdata = data.frame(L2=L2_sam))

  reg1=((L1_sam<=250)-as.numeric(contra1_sam>0))*(250-L1_sam)
  reg2=((L2_sam<=360)-as.numeric(contra2_sam>0))*(720-2*L2_sam)
  Y=rnorm(B,mean=400+1.6*L1_sam,sd=60)-reg1-reg2
  #return(c(mean(400+1.6*L1_sam-reg1-reg2),mean(Y)))
  return(mean(Y))
}
```

```
mean.opt.tree(tree1pw,tree2pw,B) ##causal tree
```

```
## [1] 1118.79
```

## 2. Example code for simulation studies in Section 4.2

```
mean.opt=function(par,B){## parameters should be passed in order.
  set.seed(1)
  ###stage 1
  W_sam=rtnorm(B,mu=45,sd=10,lb=10,ub=Inf) ##e.g., age
  L11_sam=rtnorm(B,mu=20,sd=5,lb=0,ub=Inf)##the higher, the worse.
  L12_sam=rtnorm(B,mu=10,sd=3,lb=0,ub=Inf)
  blip_mat1=rbind(numeric(B)+1,L11_sam,L12_sam)
  contra1=c(t(blip_mat1)%*%par[c(1:3)])

  ###stage 2
  L21_sam=rtnorm(B,mu=1.25*L11_sam-2*as.numeric(contra1>0),
    sd=5,lb=0,ub=Inf)
  L22_sam=rtnorm(B,mu=L12_sam-as.numeric(contra1>0),sd=3,
    lb=0,ub=Inf)
  blip_mat2=rbind(numeric(B)+1,L21_sam,L22_sam)
  contra2=c(t(blip_mat2)%*%par[c(4:6)])

  ###stage 3
  L31_sam=rtnorm(B,mu=L21_sam-2*(as.numeric(contra2>0)+as.numeric(contra1>0)),
    sd=5,lb=0,ub=Inf)
  L32_sam=rtnorm(B,mu=L22_sam-as.numeric(contra2>0),sd=3,
    lb=0,ub=Inf)
  blip_mat3=rbind(numeric(B)+1,L31_sam,L32_sam)
  contra3=c(t(blip_mat3)%*%par[c(7:9)])
}
```

```

reg1=(as.numeric((L11_sam>30)|(L12_sam>12))-as.numeric(contral>0))^2*
  (abs(L11_sam-30)+abs(L12_sam-12))/2
reg2=(as.numeric((L21_sam>25)|(L22_sam>10))-as.numeric(contral2>0))^2*
  (abs(L21_sam-25)+abs(L22_sam-10))
reg3=(as.numeric((L31_sam+L32_sam)>35)-as.numeric(contral3>0))^2*log(W_sam)*2

Y=rnorm(B,mean=100,sd=10)-reg1-reg2-reg3
return(mean(Y))
}

mean.opt.tree=function(tree1,tree2,tree3,B){ # par should be in order
  set.seed(1)
  ###stage 1
  W_sam=rtnorm(B,mu=45,sd=10,lb=10,ub=Inf) ##e.g., age
  L11_sam=rtnorm(B,mu=20,sd=5,lb=0,ub=Inf)##the higher, the worse.
  L12_sam=rtnorm(B,mu=10,sd=3,lb=0,ub=Inf)
  contral1=predict(tree1,newdata = data.frame(W=W_sam,L11=L11_sam,L12=L12_sam))

  ###stage 2
  L21_sam=rtnorm(B,mu=1.25*L11_sam-2*as.numeric(contral1>0),
    sd=5,lb=0,ub=Inf)
  L22_sam=rtnorm(B,mu=L12_sam-as.numeric(contral1>0),sd=3,
    lb=0,ub=Inf)
  contral2=predict(tree2,newdata = data.frame(W=W_sam,L21=L21_sam,L22=L22_sam))

  ###stage 3
  L31_sam=rtnorm(B,mu=L21_sam-2*(as.numeric(contral2>0)+as.numeric(contral1>0)),
    sd=5,lb=0,ub=Inf)
  L32_sam=rtnorm(B,mu=L22_sam-as.numeric(contral2>0),sd=3,
    lb=0,ub=Inf)
  contral3=predict(tree3,newdata = data.frame(W=W_sam,L31=L31_sam,L32=L32_sam))

  reg1=(as.numeric((L11_sam>30)|(L12_sam>12))-as.numeric(contral1>0))^2*
    (abs(L11_sam-30)+abs(L12_sam-12))/2
  reg2=(as.numeric((L21_sam>25)|(L22_sam>10))-as.numeric(contral2>0))^2*
    (abs(L21_sam-25)+abs(L22_sam-10))
  reg3=(as.numeric((L31_sam+L32_sam)>35)-as.numeric(contral3>0))^2*log(W_sam)*2

  Y=rnorm(B,mean=100,sd=10)-reg1-reg2-reg3
  return(mean(Y))
}

sim.case2=function(s,n_tra,n_tes,B){
  set.seed(s)
  print(s)
  ##Generate data.
  n=n_tra+n_tes
  ###stage 1
  W=rtnorm(n,mu=45,sd=10,lb=10,ub=Inf) ##e.g., age
  L11=rtnorm(n,mu=20,sd=5,lb=0,ub=Inf)##the higher, the worse.
  L12=rtnorm(n,mu=10,sd=3,lb=0,ub=Inf)
  A1=rbinom(n,1,expit(-3+0.1*W))

```



```

####stage 2
L21=rtnorm(n,mu=1.25*L11-2*A1,sd=5,lb=0,ub=Inf)
L22=rtnorm(n,mu=L12-A1,sd=3,lb=0,ub=Inf)
A2=rbinom(n,1,expit(-1+0.04*(L21+L22)))

####stage 3
L31=rtnorm(n,mu=L21-2*(A2+A1),sd=5,lb=0,ub=Inf)
L32=rtnorm(n,mu=L22-A2,sd=3,lb=0,ub=Inf)
A3=rbinom(n,1,expit(-2+0.1*L31))
####outcome:the higher, the better.
Y=rnorm(n,mean=100,sd=10)-
  (as.numeric((L11>30)|(L12>12))-A1)^2*(abs(L11-30)+abs(L12-12))/2-
  (as.numeric((L21>25)|(L22>10))-A2)^2*(abs(L21-25)+abs(L22-10))-
  (as.numeric((L31+L32)>35)-A3)^2*log(W)*2

data_all=data.frame(W=W,L11=L11,L12=L12,A1=A1,L21=L21,L22=L22,A2=A2,L31=L31,L32=L32,A3=A3,Y=Y)
data_tra=data_all[1:n_tra,]
data_tes=data_all[-c(1:n_tra),]

#####treatment model estimated from the training set
trt_1=glm(A1~L11+L12+W,family = binomial,data = data_tra)
trt_2=glm(A2~L21+L22+W,family = binomial,data = data_tra)
trt_3=glm(A3~L31+L32+W,family = binomial,data = data_tra)

pre_trt_1=predict(trt_1,type = "response")
pre_trt_2=predict(trt_2,type = "response")
pre_trt_3=predict(trt_3,type = "response")

#####Causal Tree
#####Build the Tree based on training set
tree3=causalTree(Y~W+L31+L32,treatment = A3, data=data_tra,
  weights = abs(A3 - pre_trt_3),
  split.Rule = "CT", cv.option = "CT", split.Honest = T,
  cv.Honest = T, split.Bucket = T,
  xval = 5, cp = 0, minsize = 5)

#rpart.plot(tree3)
contra3_tree=predict(tree3)

Y_opt3=data_tra$Y+((contra3_tree>0)-data_tra$A3)*contra3_tree
data_tra$Y_opt3=Y_opt3
tree2=causalTree(Y_opt3~W+L21+L22, treatment = A2, data=data_tra,
  weights = abs(A2 - pre_trt_2),
  split.Rule = "CT", cv.option = "CT", split.Honest = T,
  cv.Honest = T, split.Bucket = T,
  xval = 5, cp = 0,minsize=5)

contra2_tree=predict(tree2)

Y_opt2=data_tra$Y_opt3+((contra2_tree>0)-data_tra$A2)*contra2_tree
data_tra$Y_opt2=Y_opt2
tree1=causalTree(Y_opt2~W+L11+L12, treatment = A1, data=data_tra,

```

```

        weights = abs(A1 - pre_trt_1),
        split.Rule = "CT", cv.option = "CT", split.Honest = T,
        cv.Honest = T, split.Bucket = T,
        xval = 5, cp = 0,minsize=5)

mean_opt_tree=mean.opt.tree(tree1,tree2,tree3,B)

#####A-learning
blip.mod=list(~L11+L12,~L21+L22,~L31+L32)
treat.mod=list(A1~L11+L12+W,A2~L21+L22+W,A3~L31+L32+W)
tf.mod=list(~W+L11+L12, ~W+L11+L12+A1+A1:L11+A1:L12+L21+L22,
            ~W+L11+L12+A1+A1:L11+A1:L12+L21+L22+A2+A2:L21+A2:L22+L31+L32)

res_dr=DTRreg(data_tra$Y, blip.mod,treat.mod,tf.mod,data=data_tra,
              method = "gest",var.estim = "sandwich")
psi_dr=unlist(res_dr$psi)
mean_opt_dr=mean.opt(psi_dr,B)

#####Q-learning
res_q=DTRreg(data_tra$Y, blip.mod, treat.mod,tf.mod,data=data_tra,
             method = "qlearn",var.estim = "none")
psi_q=unlist(res_q$psi)
mean_opt_q=mean.opt(psi_q,B)

#####assess the performance of each method on the testing set
opt1=as.numeric((data_tes$L11>30)|(data_tes$L12>12))
opt2=as.numeric((data_tes$L21>25)|(data_tes$L22>10))
opt3=as.numeric((data_tes$L31+data_tes$L32)>35)

###assess the performance of causal tree
contra1_tree=predict(tree1,newdata = data_tes)
contra2_tree=predict(tree2,newdata = data_tes)
contra3_tree=predict(tree3,newdata = data_tes)
###decision accuracy of causal tree
accu1=mean(opt1==as.numeric(contra1_tree>0))
accu2=mean(opt2==as.numeric(contra2_tree>0))
accu3=mean(opt3==as.numeric(contra3_tree>0))

accu=mean((opt1==as.numeric(contra1_tree>0))&(opt2==as.numeric(contra2_tree>0))
          &(opt3==as.numeric(contra3_tree>0)))

###assess the performance of A-learning
blip_mat1=rbind(numeric(n_tes)+1,data_tes$L11,data_tes$L12)
blip_mat2=rbind(numeric(n_tes)+1,data_tes$L21,data_tes$L22)
blip_mat3=rbind(numeric(n_tes)+1,data_tes$L31,data_tes$L32)

contra1_dr=t(blip_mat1)%*%psi_dr[c(1:3)]
contra2_dr=t(blip_mat2)%*%psi_dr[c(4:6)]
contra3_dr=t(blip_mat3)%*%psi_dr[c(7:9)]
###decision accuracy of A-learning
accu1_dr=mean(opt1==as.numeric(contra1_dr>0))
accu2_dr=mean(opt2==as.numeric(contra2_dr>0))
accu3_dr=mean(opt3==as.numeric(contra3_dr>0))

```

```

accu_dr=mean((opt1==as.numeric(contra1_dr>0))&(opt2==as.numeric(contra2_dr>0))&
              (opt3==as.numeric(contra3_dr>0)))

###assess the performance of Q-learning
contra1_q=t(blip_mat1)%*%psi_q[c(1:3)]
contra2_q=t(blip_mat2)%*%psi_q[c(4:6)]
contra3_q=t(blip_mat3)%*%psi_q[c(7:9)]
###decision accuracy of Q-learning
accu1_q=mean(opt1==as.numeric(contra1_q>0))
accu2_q=mean(opt2==as.numeric(contra2_q>0))
accu3_q=mean(opt3==as.numeric(contra3_q>0))

accu_q=mean((opt1==as.numeric(contra1_q>0))&(opt2==as.numeric(contra2_q>0))
              &(opt3==as.numeric(contra3_q>0)))

return(list(Tree=c(accu1,accu2,accu3,accu,mean_opt_tree),
                  Alearn=c(accu1_dr,accu2_dr,accu3_dr,accu_dr,mean_opt_dr),
                  Qlearn=c(accu1_q,accu2_q,accu3_q,accu_q,mean_opt_q)))
}

sim.case2(1,n_tra=1000,n_tes=1000,B=10000)

```

```

## [1] 1
## $Tree
## [1] 0.97500 0.99600 0.92200 0.89300 99.36644
##
## $Alearn
## [1] 0.89800 0.90200 0.97400 0.78900 98.53013
##
## $Qlearn
## [1] 0.89900 0.90200 0.97400 0.79000 98.50465

```

```

sim.case2(1,n_tra=500,n_tes=1000,B=10000)

```

```

## [1] 1
## $Tree
## [1] 0.89900 0.92600 0.81200 0.68400 97.10622
##
## $Alearn
## [1] 0.85300 0.93600 0.94600 0.75500 98.36439
##
## $Qlearn
## [1] 0.8330 0.9400 0.9470 0.7440 98.2891

```

## References

Wallace, Michael P., and Erica E. M. Moodie. 2015. “Doubly-Robust Dynamic Treatment Regimen Estimation via Weighted Least Squares.” *Biometrics* 71 (3): 636–44. <https://doi.org/10.1111/biom.12306>.
